# Supplementary material for: Deconvolutional Paragraph Representation Learning
Source: arXiv:1708.04729 source file (2017-09-22)
Supplement: Supplementary file 1 [file textCNN_supp.pdf]

## Supplementary Material for Deconvolutional Paragraph Representation Learning

**Experimental setup** For all the experiments, we use a 3-layer convolutional encoder followed by a 3-layer deconvolutional decoder. Filter size, stride and word embedding are set to  $h = 5$ ,  $r^l = 2$ , for  $l = 1, \dots, 3$  and  $k = 300$ , respectively. The dimension of the latent representation vector varies for each experiment, thus is reported separately.

We use the ADAM optimizer [55] for training. The learning rate is set to  $10^{-5}$  initially, and exponentially decreased at a rate of  $1 - 10^{-5}$  per iteration. The batchsize for different tasks ranges from 16 to 64. As recommended by previous work [24], we adopt gradient clipping and batch normalization techniques to stabilize model training. We initialized the weights using Xavier [56]. All embeddings are initialized uniformly within  $[-0.001, 0.001]$ . All experiments were performed using two NVIDIA GeForce GTX TITAN X GPUs.

For CNN-LSTM, the architecture of the encoder is identical to that of CNN-DCNN, while the LSTM decoder shares embedding matrix,  $\mathbf{W}_e$ , with the CNN. The number of hidden units in all LSTM encoders and decoders is set to the dimension of  $\mathbf{h}$ . To alleviate exposure bias, all LSTM decoders used in this work take  $\mathbf{h}$  along with the previous word as input for each time step. The LSTM encoder in LSTM-LSTM uses reversed sequences as inputs, as suggested in [47]. CNN-DCNN has the least number of parameters. For example, using 500 as the dimension of  $\mathbf{h}$  results in about 9, 13, 15 million total trainable parameters for CNN-DCNN, CNN-LSTM and LSTM-LSTM, respectively.

**Computational time for hotel review reconstruction** For hotel review reconstruction, the computational time for CNN-DCNN with 1 epochs is 57 minutes. CNN-LSTM takes 152 minutes and LSTM-LSTM takes 238 minutes. The memory usage of LSTM-LSTM is around 1.8 times larger than CNN-DCNN, and CNN-LSTM is around 1.5 times larger than CNN-DCNN. All evaluations are done on one single Titan X GPU.

**Character-level correction dataset and experimental setups**, which contains the top 10 largest main categories of Yahoo! Answers Comprehensive Questions and Answers. We use the question content field of the dataset. Questions shorter than 5 words or longer than 300 are excluded during preprocessing. Training, validation and testing sets consist of 110000, 124768, 52437 sentences, respectively, randomly chosen from the full set.

**Actor-critic experimental setups** We use the original code of [53], with their reported best configuration (actor-critic + log-likelihood training). The probability of substitution is set to be 0.3, and the clip length is set to be 30 (as default). The algorithm was running for 100,000 iteration and reached convergence (for around 20 hours). We test on the held-out dataset and report the mean CER. We did not run a configuration with maximum length of characters as clip length, in our case, 300. For the sentences with more than 30 characters, such as  $L$ , when evaluate actor-critic, we use a sliding window of 30 characters to perform  $L - 30 + 1$  tests of actor-critic evaluation and use the most voted character over all  $L - 30 + 1$  tests for final output. In general when setting the clip length to a larger value, the performance decreases, thus we expect with a even longer clip length the actor-critic algorithm may perform worse than current setup.

**Additional character-level correction results** See Figure ?? for more examples of character-level correction.

|             |                                           |             |                                           |
|-------------|-------------------------------------------|-------------|-------------------------------------------|
| Original    | does anyone else think chris own is hot ? | Original    | how do you delete your computer history ? |
| Modified    | dchz nnyond elae bhink chrig own is hot f | Modified    | hlw do yow delete yhur cempcthr histry ?  |
| ActorCritic | does anyone elat think chrig own is hot f | ActorCritic | how do you delete your cemp tor history ? |
| CNN-LSTM    | does anyone else thin charg for in so ?   | CNN-LSTM    | how do you delete you penterce history ?  |
| CNN-DCNN    | does anyone else think chris own is hot ? | CNN-DCNN    | how do you delete your computer history ? |

Figure 6: Additional Character-level correction

**Word-level correction results** We consider an arXiv dataset for word-level correction, which consists of 0.8 million sentences from the abstracts of papers from various subjects, obtained from the arXiv website. Sentences exceeding 60 words are excluded during preprocessing. We randomly choose 750000, 20000, 10000 sentences to construct our training, validation and testing sets. We use this dataset because arXiv sentences are relatively longer than Yahoo dataset. For word-level correction we set the dimension of  $h$  to 500. We consider both solely word substitution (with 30% words substituted), and mixed perturbations with three sources: word substitution, deletion and insertion (with 20% words substituted, 5% added and 5% deleted). Generally, CNN-DCNN outperforms CNN-LSTM and LSTM-LSTM and converges faster. We provide the comparative results in Figure ?? and Figure ?. The correction results for word substitution are shown in Table ?. For this task, LSTM-LSTM is around 3 times slower than CNN-DCNN and CNN-LSTM is around 2.5 times slower. The memory usage of CNN-DCNN is around half of the memory usage comparing to LSTM-LSTM.

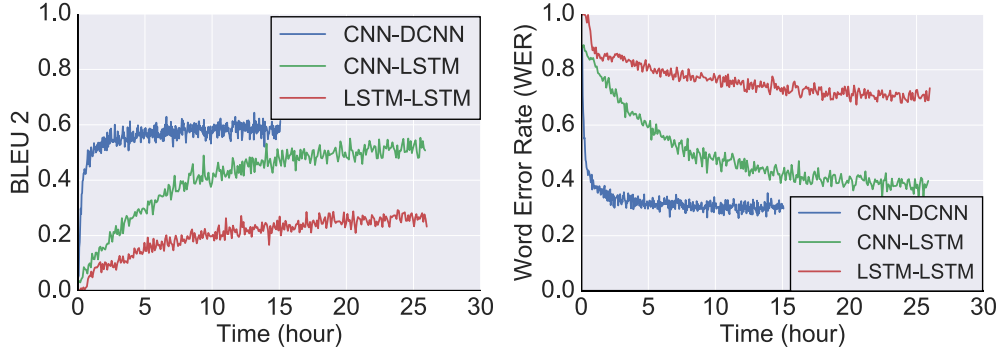

Figure 7: BLEU and Word Correction Rate for substitution error. Left: BLEU-2 score comparison. Right: Word-level Error Rate(WER)

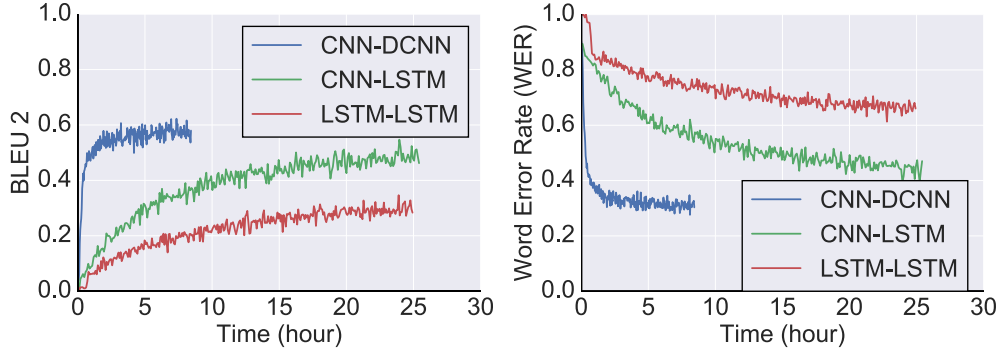

Figure 8: BLEU and Word Correction Rate for mixed error. Left: BLEU-2 score comparison. Right: Word-level Error Rate(WER)

**Dataset detail for sequence classification** The details for semi-supervised sequence classification datasets are provided in Table ??.

**Semi-supervised results for DBpedia and Yahoo Answer Dataset** We report the results for DBpedia and Yahoo dataset as in Table ?? and Table ??.

**Summarization discussions and results** We provide several examples for our summarization results in Table ?. Generally, an LSTM decoder with joint training achieves most compelling summarization of the arXiv abstract, and tends to utilize the words that appears in the abstract. Deconvolutional decoder receives reasonably high Rouge and BLEU score (see Table ?), however the generated text is less coherent. As discussed in Section 2, a deconvolutional decoder is essentially stacking text segments when composing a model output. This would be preferable for reconstructing,

Table 6: Word-level correction results with substitution errors. The first shown case is with sole substitution, the second shown case is with mixed modification. LSTM-LSTM are not shown because it is not comparable to CNN-LSTM.

|                      |                                                                                                       |
|----------------------|-------------------------------------------------------------------------------------------------------|
| <b>Ground Truth:</b> | this paper proposes a parametric approach for stochastic modeling of limit order markets .            |
| <b>Modified:</b>     | this limbs guarding form parametric approach for stochastic modeling screwing limit trickle markets . |
| <b>CNN-LSTM:</b>     | this paper presents the new approach for stochastic modeling model in n .                             |
| <b>LSTM-LSTM:</b>    | however , it is important to solve this problem in a bayesian framework of learning parameters .      |
| <b>CNN-DCNN:</b>     | this paper provides a parametric approach for stochastic modeling to study the markets .              |

  

|                      |                                                                                           |
|----------------------|-------------------------------------------------------------------------------------------|
| <b>Ground Truth:</b> | i caught hold of the counter 's edge , using it to keep me upright .                      |
| <b>Modified:</b>     | i caught industries the counter 's lognormal edge , using rewarded to convex me upright . |
| <b>LSTM-LSTM:</b>    | i 'm sure i heard in the UNK 's hand off , ready to wait for me to .                      |
| <b>CNN-LSTM:</b>     | i caught on the counter 's edge edge , using him to feed me down .                        |
| <b>CNN-DCNN:</b>     | i caught out of the counter 's edge , using it to leave me upright .                      |

Table 7: Summary statistics for benchmark document classification datasets.

| Dataset      | Classes | Train     | Test   | Average#w | Vocabulary |
|--------------|---------|-----------|--------|-----------|------------|
| DBpedia      | 14      | 560,000   | 70,000 | 57        | 21,666     |
| Yelp P.      | 2       | 560,000   | 38,000 | 138       | 25,709     |
| Yahoo Answer | 10      | 1,400,000 | 60,000 | 104       | 39,428     |

Table 8: Semi-supervised classification results on DBpedia with different proportions of labeled data.

| Model                        | 0.1%  | 1%    | 10%  | 100% |
|------------------------------|-------|-------|------|------|
| Purely supervised            | 66.07 | 19.39 | 3.62 | 1.76 |
| Joint training with CNN-LSTM | 47.32 | 12.27 | 3.37 | 1.36 |
| Joint training with CNN-DCNN | 37.59 | 10.08 | 2.73 | 1.17 |

Table 9: Semi-supervised classification results on Yahoo Answer Dataset with different proportions of labeled data.

| Model                        | 0.1%  | 1%    | 10%   | 100%  |
|------------------------------|-------|-------|-------|-------|
| Purely supervised            | 82.58 | 46.65 | 32.25 | 27.42 |
| Joint training with CNN-LSTM | 48.40 | 35.45 | 28.78 | 26.32 |
| Joint training with CNN-DCNN | 42.51 | 31.28 | 27.07 | 25.82 |

Table 10: Quantitative results using BLEU-2 and ROUGE-L.

| Method                                   | BLEU-2      | ROUGE-L      |
|------------------------------------------|-------------|--------------|
| sup CNN-RNN ( $\sigma = 5\%$ )           | 2.40        | 12.40        |
| semi-sup CNN-RNN ( $\sigma = 5\%$ )      | 3.58        | 16.04        |
| sup CNN-RNN ( $\sigma = 10\%$ )          | 2.66        | 13.07        |
| semi-sup CNN-RNN ( $\sigma = 10\%$ )     | 3.86        | 16.62        |
| sup CNN-RNN ( $\sigma = 50\%$ )          | 3.68        | 15.87        |
| semi-sup CNN-RNN ( $\sigma = 50\%$ )     | 4.16        | 17.64        |
| sup CNN-RNN ( $\sigma = 100\%$ )         | 4.18        | 16.37        |
| semi-sup CNN-RNN ( $\sigma = 100\%$ )    | <b>5.28</b> | <b>18.14</b> |
| sup CNN-Deconv ( $\sigma = 100\%$ )      | 2.12        | 14.75        |
| semi-sup CNN-Deconv ( $\sigma = 100\%$ ) | 2.82        | 16.83        |

since the input-output pair is unique. However for tasks like summarization, translation and image captioning, each input may correspond to multiple plausible output sequences. Under these scenarios, it is challenging for a deconvolutional decoder to decide where to put the text fragments, as the conditional information is weaker than RNN-based strategies.

Table 11: Summary results

|                     |                                                                                                                                                                                                                                                                                                                                                                                                                                                                                                                                                                                                                                                                                                                                                                                                                                                                                                                                                                                                                                         |
|---------------------|-----------------------------------------------------------------------------------------------------------------------------------------------------------------------------------------------------------------------------------------------------------------------------------------------------------------------------------------------------------------------------------------------------------------------------------------------------------------------------------------------------------------------------------------------------------------------------------------------------------------------------------------------------------------------------------------------------------------------------------------------------------------------------------------------------------------------------------------------------------------------------------------------------------------------------------------------------------------------------------------------------------------------------------------|
| Abstract:           | this paper presents a new state of the art for document image classification and retrieval , using features learned by deep convolutional neural networks ( cnns ) . in object and scene analysis , deep neural nets are capable of learning a hierarchical chain of abstraction from pixel inputs to concise and descriptive representations . the current work explores this capacity in the realm of document analysis , and confirms that this representation strategy is superior to a variety of popular hand crafted alternatives . experiments also show that ( i ) features extracted from cnns are robust to compression , ( ii ) cnns trained on non document images transfer well to document analysis tasks , and ( iii ) enforcing region specific feature learning is unnecessary given sufficient training data . this work also makes available a new labelled subset of the <UNK> <UNK> collection , containing 400 , 000 document images across 16 categories , useful for training new cnns for document analysis . |
| Ground-truth        | evaluation of deep convolutional nets for document image classification and retrieval                                                                                                                                                                                                                                                                                                                                                                                                                                                                                                                                                                                                                                                                                                                                                                                                                                                                                                                                                   |
| Sup LSTM decoder:   | deep learning for image recognition                                                                                                                                                                                                                                                                                                                                                                                                                                                                                                                                                                                                                                                                                                                                                                                                                                                                                                                                                                                                     |
| Joint LSTM decoder: | a classification algorithm for deep neural networks                                                                                                                                                                                                                                                                                                                                                                                                                                                                                                                                                                                                                                                                                                                                                                                                                                                                                                                                                                                     |
| Sup DCNN decoder:   | <UNK> deep neural convolutional for for recognition                                                                                                                                                                                                                                                                                                                                                                                                                                                                                                                                                                                                                                                                                                                                                                                                                                                                                                                                                                                     |
| Joint DCNN decoder: | residual and based neural based classification for recognition network                                                                                                                                                                                                                                                                                                                                                                                                                                                                                                                                                                                                                                                                                                                                                                                                                                                                                                                                                                  |
| Abstract:           | the 2 ms chandra deep field north survey provides the deepest view of the universe in the 0 . 5 8 . 0 kev x ray band . in this brief review we investigate the diversity of x ray selected sources and focus on the constraints placed on agns ( including binary agns ) in high redshift submm galaxies .                                                                                                                                                                                                                                                                                                                                                                                                                                                                                                                                                                                                                                                                                                                              |
| Ground-truth        | the 2 ms chandra deep field north moderate luminosity agns and dusty starburst galaxies                                                                                                                                                                                                                                                                                                                                                                                                                                                                                                                                                                                                                                                                                                                                                                                                                                                                                                                                                 |
| Sup LSTM decoder:   | the infrared evolution of the x ray galaxies in the deep field                                                                                                                                                                                                                                                                                                                                                                                                                                                                                                                                                                                                                                                                                                                                                                                                                                                                                                                                                                          |
| Joint LSTM decoder: | the x ray luminosity function of the chandra deep field                                                                                                                                                                                                                                                                                                                                                                                                                                                                                                                                                                                                                                                                                                                                                                                                                                                                                                                                                                                 |
| Sup DCNN decoder:   | the deep infrared ray galaxies of the the <UNK>                                                                                                                                                                                                                                                                                                                                                                                                                                                                                                                                                                                                                                                                                                                                                                                                                                                                                                                                                                                         |
| Joint DCNN decoder: | faint deep infrared field galaxies of the clusters hubble revealed                                                                                                                                                                                                                                                                                                                                                                                                                                                                                                                                                                                                                                                                                                                                                                                                                                                                                                                                                                      |
| Abstract:           | we study spatial correlations in the transport of energy between two baths at different temperatures . to do this , we introduce a minimal model in which energy flows from one bath to another through two subsystems . we show that the transport induced energy correlations between the two subsystems are of the same order as the energy fluctuations within each subsystem . the correlations can be either positive or negative and we give bounds on their values which are associated with a dynamic energy scale . the different signs originate as a competition between fluctuations generated near the baths , and fluctuations of the current between the two subsystems . this interpretation sheds light on known results for spatially dependent heat and particle conduction models .                                                                                                                                                                                                                                |
| Ground-truth        | transport induced correlations in weakly interacting systems                                                                                                                                                                                                                                                                                                                                                                                                                                                                                                                                                                                                                                                                                                                                                                                                                                                                                                                                                                            |
| Sup LSTM decoder:   | classical quantum field of with correlations quantum field model surface                                                                                                                                                                                                                                                                                                                                                                                                                                                                                                                                                                                                                                                                                                                                                                                                                                                                                                                                                                |
| Joint LSTM decoder: | transport in the particle transport in a two dimensional spin                                                                                                                                                                                                                                                                                                                                                                                                                                                                                                                                                                                                                                                                                                                                                                                                                                                                                                                                                                           |
| Sup DCNN decoder:   | a new model of the <UNK> <UNK>                                                                                                                                                                                                                                                                                                                                                                                                                                                                                                                                                                                                                                                                                                                                                                                                                                                                                                                                                                                                          |
| Joint DCNN decoder: | classical quantum field of with correlations quantum field model surface                                                                                                                                                                                                                                                                                                                                                                                                                                                                                                                                                                                                                                                                                                                                                                                                                                                                                                                                                                |
